# Supplementary material for: Zigzag chain order of LiVSe$_2$ developing away from the vanadium trimer phase transition boundary
Source: arXiv:2309.11749 source file (2023-09-21)
Supplement: Supplementary file 1 [file LiVSe2_supplement_3.pdf]

# Supplemental material of "Zigzag chain order of $LiVSe_2$ developing away from the vanadium trimer phase transition boundary"

K. Kojima,[1] N. Katayama,[1,*] K. Sugimoto,[2] N. Hirao,[3] Y. Ohta,[4] and H. Sawa[1]

[1]*Department of Applied Physics, Nagoya University, Nagoya 464-8603, Japan*
[2]*Department of Physics, Keio University, Kanagawa 223-8522, Japan*
[3]*Diffraction and Scattering Division, Center for Synchrotron Radiation, Japan Synchrotron Radiation Research Institute, Hyogo 679-5198, Japan*
[4]*Department of Physics, Chiba University, Chiba 263-8522, Japan*

(Dated: June 30, 2023)

## I. MAGNETIC SUSCEPTIBILITY

The magnetic susceptibilities of our samples are shown in Fig. S 1(a). Magnetization measurements were performed on the sample wrapped in aluminum foil under a magnetic field of 1T. The magnetization measurement of the aluminum foil was then performed under similar conditions, and the data was subtracted to obtain the magnetization of the sample. Curie tail was estimated by Curie fitting, which includes a constant term for temperature, for the temperature range from 2 K to 40 K. The experimental results minus the Curie tail are shown in Fig. S 1(b). The increase in magnetic susceptibility with increasing temperature can be clearly seen.

It should be mentioned that a similar positive temperature dependence of magnetic susceptibility is also observed in the high-temperature phase of $LiVS_2$ [9]. This temperature dependence of magnetic susceptibility has been reported as pseudogap behavior in a previous paper [9] and discussed in a follow-up paper as being associated with the development of zigzag chains [28]. The temperature dependence of the magnetic susceptibility of $LiVSe_2$ is expected to be interpreted in the same way, so the pseudogap phase of the $LiVX_2$ system should be realized corresponding to the zigzag chain phase shown in green in Fig. 1 in the main article.

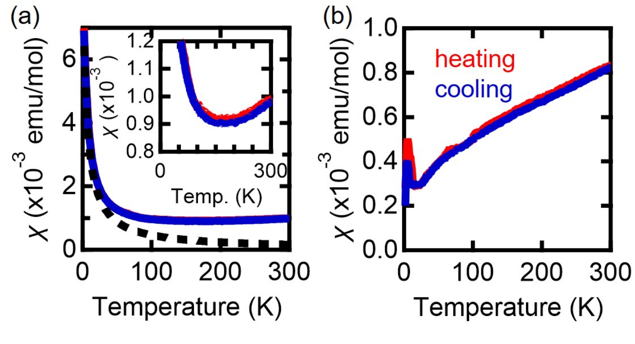


FIG. S 1. (a) Raw data of magnetic susceptibility. Curie tail fitting is indicated by black dotted lines. The inset shows an enlarged figure. (b) Magnetic susceptibility subtracted the results of Curie fitting.

* Corresponding author.; katayama.naoyuki.m5@f.mail.nagoya-u.ac.jp

## II. CORRECTION OF XRD DATA OBTAINED AT BEAMLINE BL44B2

At SPring-8 BL44B2, diffraction data are collected using several 1D semiconductor detectors called MYTHEN. The detector has many semiconductor modules in a row. However, because of manufacturing irregularities between the semiconductors, even x-rays with the same photon number will have different intensity data depending on which module they are detected by. Therefore, to obtain highly accurate experimental data, it is necessary to compensate for the irregularities between modules to minimize systematic errors.

Generally, manufacturers implement a "flat field correction" for such irregularities. However, because the sensitivity irregularities of detectors vary with x-ray energy and temperature changes, the manufacturer's correction may not be sufficient. Therefore, a calibration system has been constructed at BL44B2 at SPring-8 that corrects for irregularities between elements through statistical processing [31,32]. This allows us to implement corrections according to the experimental environment at the time, improving the data's accuracy. Therefore, we corrected the experimental data based on the system provided at BL44B2.

## III. RESULTS OF RIETVELD ANALYSIS AT AMBIENT PRESSURE

The $R$ values obtained from the Rietveld analysis shown in Figure 2(a,b) in the main text, which indicate the degree of agreement of the analysis, are respectively as follows. (a) $R_{wp}$ = 3.216%, $R_p$ = 2.601%, $R_e$ = 0.344%, $S$ = 9.3355, and (b) $R_{wp}$ = 2.528%, $R_p$ = 2.130%, $R_e$ = 0.345%, $S$ = 7.3483. Although $R_{wp}$ and $R_p$ show good values, the $R_e$ indicating statistical accuracy of experimental data is small, so $S$ becomes large by the equation $S = R_{wp}/R_e$. We would like to add that this does not mean that the analysis is not working. The structural parameters obtained by Rietveld analysis assuming a zigzag chain structure (space group $Pm$) for

TABLE S I. Atomic coordinates of zigzag chain structure obtained by Rietveld analysis of 100 K diffraction data at ambient pressure. The lattice parameters are $a_{\rm m}$ = 6.2407(6) Å, $b_{\rm m}$ = 3.5632(3) Å, $c_{\rm m}$ = 6.3425(2) Å, $\beta$ = 89.884(14) deg., $\alpha$ = $\gamma$ = 90 deg.

| | atomic coordinates | | | |
|---|---|---|---|---|
| atom | $x$ | $y$ | $z$ | $B_{iso}$ (Å) |
| V | 0 | 0 | 0 | 0.17(4) |
| V | 0.4429(10) | 1/2 | 0 | 0.17(4) |
| Se | 0.6402(19) | 0 | 0.7634(12) | 0.110(17) |
| Se | 0.1510(20) | 1/2 | 0.7583(13) | 0.110(17) |
| Se | 0.8028(20) | 1/2 | 0.2113(12) | 0.110(17) |
| Se | 0.3057(20) | 0 | 0.2574(12) | 0.110(17) |
| Li | 0 | 0 | 1/2 | 1.0 |
| Li | 1/2 | 1/2 | 1/2 | 1.0 |

100 K data are shown in Table S I. The temperature factor could not be refined well due to the high background, so it was fixed for each element.

## IV. ANALYSIS METHOD FOR DIFFRACTION DATA UNDER PRESSURE

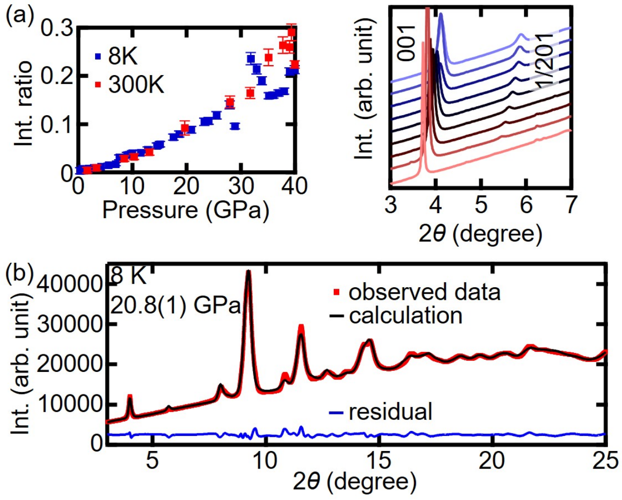


FIG. S 2. (a) Pressure dependence of the intensity ratios of the fundamental peak (001) and zigzag chain structure peak ($\frac{1}{2}$01). (b) Results of Rietveld analysis at 8 K, 20.8(1) GPa.

As shown in Fig. 4(a) of the main article, the superlattice peak at $\frac{1}{2}$01, which suggests the appearance of zigzag chains, becomes more apparent by increasing pressure. The pressure dependence of the ratio of the intensity of the superlattice peaks to the 001 fundamental peaks is shown in Fig. S 2(a), which monotonically increases by increasing pressure. This indicates that the atomic displacement of vanadium increases under pressure. On the other hand, it should be mentioned that it is difficult to determine the displacement of vanadium in all pressure regions from the Rietveld analysis. This is because the background intensity is significantly larger than the peak intensity due to x-ray fluorescence (especially Se) and scattering by the window material of the diamond anvil cell and cryostat. Another reason is that the crystallinity decreases under pressure, which worsens the peak profile.

TABLE S II. The $R$ values are as follows, $R_{wp} = 1.737\%$, $R_p = 1.134\%$, $R_e = 0.745\%$, $S = 2.3298$. The lattice parameters are $a_{\rm m}$ = 5.8359(6) Å, $b_{\rm m}$ = 3.273(3) Å, $c_{\rm m}$ = 5.9233(7) Å, $\alpha = \beta$ = $\gamma$ = 90 deg. Monoclinic $\beta$ was fixed at 90 deg. because the error was very large due to the worsening diffraction profile.

| | atomic coordinates | | |
|---|---|---|---|
| atom | $x$ | $y$ | $z$ |
| V | 0 | 0 | 0 |
| V | 0.4114(20) | 1/2 | 0 |
| Se | 0.63(4) | 0 | 0.775(15) |
| Se | 0.124(21) | 1/2 | 0.696(15) |
| Se | 0.78(3) | 1/2 | 0.0.230(15) |
| Se | 0.292(21) | 0 | 0.300(15) |
| Li | 0 | 0 | 1/2 |
| Li | 1/2 | 1/2 | 1/2 |

Therefore, in this study, the displacement of vanadium under pressure was estimated by the following procedure. First, Rietveld analysis was performed assuming the monoclinic space group $Pm$ for the data at 20.8(1) GPa, where the peak shape is relatively sharp and the superlattice peak is clearly observed. The result of the Rietveld analysis is shown in Fig. S 2(b), and the atomic coordinates obtained from this structural analysis are shown in Table S II Based on this data, the direction of atomic displacement of each element due to pressure application becomes clear. Assuming that only the magnitude of displacement changes while the direction of atomic displacement of each element is maintained when the pressure is increased or decreased, we simulated the amount of atomic displacement in each pressure region such that the value of Int.$_{\frac{1}{2}01}$ / Int.$_{001}$ shown in Fig. S 2(a) is obtained. The main article's data in Fig. 4(d) were obtained. Therefore, although the V-V displacements shown in Fig. 4(d) were obtained by simulations based on experimental data except for the value at 20.8(1) GPa, the data show changes consistent with the trend of the Int.$_{\frac{1}{2}01}$ / Int.$_{001}$ value, and we would like to emphasize that the argument in this paper is valid.
